# Supplementary material for: IBADR: an Iterative Bias-Aware Dataset Refinement Framework for Debiasing NLU models
Source: arXiv:2311.00292 source file (2023-11-01)
Supplement: Supplementary file 1 [file appendix.tex]

\section{Quality Assessment of Generated Pseudo Samples}
% We initially follow the method described in \cite{wu2022generating} to filter the generated pseudo-samples. Afterward, 
One hundred samples were randomly selected from the sample pool. Three human annotators were tasked with manually categorizing the relationships between sentence pairs within these samples. Annotations underwent a rigorous validation process through majority voting, resulting in an accuracy rate of 92\% for the pseudo samples. This accuracy was determined based on human-annotated gold labels.

\section{Exploring \model compatibility with Larger Language Models}
\label{apdx:lora}
To ensure a valid comparison with the $z$-filter, we employ GPT-2 Large as the sample generator in our main study. To explore the integration of IBADR with larger models, we fine-tune the LLaMA-7b model \cite{llama} using LORA \cite{hu2021lora} as an alternative to GPT-2 large. The results of this exploration of the MNLI dataset are listed in Table \ref{tab:lora}. From the table, we can observe the performance of \model gets further improved with the more powerful language model LLaMA-7b, which indicates \model's generalizability. 

\begin{table}[th]
\centering
\resizebox{\columnwidth}{!}{
\begin{tabular}{l|ccc}
\toprule
\multirow{2}{*}{\textbf{Data}} & \multicolumn{3}{c}{\textbf{MNLI}}                                         \\ \cline{2-4} 
                  & \multicolumn{1}{c}{dev-m} & \multicolumn{1}{c}{dev-mm} & HANS  \\ \hline
\model (GPT-2)                & 85.17	 & 85.05	& 71.67  \\
\model (LLaMA-7b)               &  85.64	& 85.81	& 72.78  \\
\bottomrule
\end{tabular}%
}
\caption{Results of \model with GPT-2 and LLaMA-7b on MNLI.}
\label{tab:lora}
\end{table}
